# Supplementary material for: Formation of Micrometer-Sized Textured Hexagonal Silicon Crystals via Nanoindentation
Source: arXiv:2410.08372 source file (2024-10-10)
Supplement: Supplementary file 1 [file Supporting_Info.pdf]

# Supplementary Material

# Formation of Micrometer-Sized Textured Hexagonal Silicon Crystals via Nanoindentation

Mouad Bikerouin[1‡], Anna Marzegalli[1‡], Davide Spirito[2], Gerald J. K. Schaffar[3], Corrado Bongiorno[4], Fabrizio Rovaris[1], Mohamed Zaghloul[4], Agnieszka Anna Corley-Wiciak[2], Leo Miglio[1], Verena Maier-Kiener[3], Giovanni Capellini[2,5*], Antonio M. Mio[4], Emilio Scalise[1*]

[1]*Department of Materials Science, University of Milano-Bicocca, Via R. Cozzi 55, I-20125, Milano, Italy*

[2]*IHP-Leibniz-Institut für innovative Mikroelektronik, Im Technologiepark 25, 15236 Frankfurt(Oder), Germany*

[3]*Department of Materials Science, Montanuniversität Leoben, Roseggerstrasse 12, 8700 Leoben, Austria*

[4]*Institute for Microelectronics and Microsystems (IMM), Consiglio Nazionale delle Ricerche (CNR), Strada VIII N. 5, 95121, Catania, Italy*

[5]*Department of Sciences, Università Roma Tre, V.le G. Marconi 446 00146, Italy*

[‡]*These authors contributed equally to this work*

[*]*Correspondence to:* emilio.scalise@unimib.it ; capellini@ihp-microelectronics.com

**Table S1.** Raman active mode frequencies (in $cm^{-1}$) of indented silicon using a 20 μm tip are presented for two distinct groups of pits, labeled as Group-I and Group-II. The identified metastable silicon phases are reported under both as-indented and post-annealed conditions. Experimental values (Exp.) are provided as reference for comparison.

| | Phase | Raman Mode | Group-I Pits: 2, 4, 5, 6, 8 | Group-II Pits: 1, 3, 7, 9 | Exp. [1] |
|---|---|---|---|---|---|
| As-indented | dc | $T_{2g}$ | 526.9 ± 2.2 | 531.9 ± 1.4 | 520 |
| | r8 | $A_g$ | 165.3 ± 0.2 | 165.1 ± 0.2 | 165 |
| | | $E_g$ | 170.7 ± 1.1 | 171.2 ± 0.4 | 170 |
| | | $A_g$ | 354.4 ± 0.6 | 354.7 ± 0.3 | 352 |
| | | $E_g$ | 375.3 ± 1.1 | 376.1 ± 1.1 | 373 |
| | | $A_g$ | 399.4 ± 0.6 | 399.9 ± 0.2 | 397 |
| | | $A_g$ | 415.3 ± 3.1 | 416.5 ± 2.6 | 413 |
| | | $E_g$ | 435.4 ± 1.8 | 438.4 ± 1.9 | 433 |
| | | $E_g$ | 494.5 ± 4.3 | 495.8 ± 2.4 | 495 |
| | bc8 | $T_g$ | 182.7 ± 0.6 | 182.9 ± 0.0 | 182 |
| | | $T_g$ | 375.3 ± 1.1 | 376.1 ± 1.1 | 373 |
| | | $A_g$ | 386.2 ± 0.8 | 387.0 ± 0.3 | 384 |
| | | $T_g$ | 441.2 ± 2.9 | 445.5 ± 2.2 | 438 |
| | | $E_g$ | 467.2 ± 4.9 | 464.8 ± 3.2 | 463 |
| Post-annealed | dc | $T_{2g}$ | 525.3 ± 3.3 | 529.2 ± 1.2 | 520 |
| | hd | $E_{2g}$ | 483.4 ± 7.0 | 492.0 ± 1.4 | 496 |
| | | $E_{1g}$ | 513.7 ± 5.9 | 524.2 ± 1.2 | 514 |
| | | $A_{1g}$ | 513.7 ± 5.9 | 524.2 ± 1.2 | 514 |

**Table S2.** Lattice constants (a and c in Å), structural parameter (c/a), equilibrium volume (V in $Å^3$/atom), bulk modulus ($B_0$ in GPa), its pressure derivative ($B_0'$), and the energy difference from the corresponding dc phase (ΔE in meV/atom) for various metastable Si phases obtained using different exchange-correlation (XC) functionals (LDA, PBE, PBEsol, and SCAN). Experimental (Exp.) and previous theoretical (Theo.) values are provided for comparison.

| Structure Space group | Method | a (Å) | c (Å) | c/a | V ($Å^3$/atom) | $B_0$ (GPa) | $B_0'$ | ΔE (meV/atom) |
|---|---|---|---|---|---|---|---|---|
| dc Fd-3m (227) | LDA | 5.395 | - | - | 19.63 | 95.6 | 4.22 | 0 |
| | PBE | 5.469 | - | - | 20.45 | 87.9 | 4.29 | 0 |
| | PBEsol | 5.431 | - | - | 20.03 | 93.0 | 4.23 | 0 |
| | SCAN | 5.412 | - | - | 19.81 | 98.3 | 4.14 | 0 |
| | Exp. [2] | 5.431 | - | - | 20.02 | 97.9 | 4.24 | 0 |
| | Theo. (PBE) [3] | - | - | - | 20.45 | 88.9 | 4.1 | 0 |
| | Theo. (LDA) [4] | 5.397 | - | - | 19.64 | 96.6 | 4.18 | 0 |
| hd $P6_3/mmc$ (194) | LDA | 3.797 | 6.282 | 1.6544 | 19.61 | 95.0 | 4.12 | 10 |
| | PBE | 3.850 | 6.364 | 1.6527 | 20.43 | 87.3 | 4.25 | 11 |
| | PBEsol | 3.823 | 6.322 | 1.6536 | 20.00 | 92.4 | 4.18 | 10 |
| | SCAN | 3.809 | 6.304 | 1.6550 | 19.80 | 98.3 | 4.11 | 9 |
| | Exp. [5] | 3.8237 | 6.3237 | 1.6538 | 20.02 | - | - | - |
| | Exp. [6] | 3.824 | 6.257 | 1.6362 | 19.81 | - | - | - |
| | Exp. [7] | 3.840 | 6.280 | 1.630 | 20.05 | - | - | - |
| | Exp. [8] | 3.837 | 6.317 | 1.646 | 20.14 | - | - | - |
| | Theo. (PBE) [3] | - | - | - | 20.43 | 88.6 | 4.4 | 11 |
| | Theo. (LDA) [4] | 3.798 | 6.280 | 1.653 | 19.61 | 96.7 | 4.06 | 10.7 |
| r8 R-3 (148) | LDA | 9.314 | 5.567 | 0.5977 | 17.43 | 86.9 | 3.80 | 121 |
| | PBE | 9.447 | 5.659 | 0.5990 | 18.22 | 78.4 | 4.17 | 160 |
| | PBEsol | 9.369 | 5.597 | 0.5975 | 17.73 | 83.4 | 4.11 | 117 |
| | SCAN | 9.377 | 5.632 | 0.6006 | 17.87 | 85.0 | 4.09 | 207 |
| | Exp. [9] | 9.402 | 5.590 | 0.5946 | 17.83 | - | - | - |
| | Theo. (PBE) [3] | - | - | - | 18.22 | 78.8 | 4.3 | 160 |
| bc8 Ia-3 (206) | LDA | 6.561 | - | - | 17.65 | 92.7 | 4.24 | 123 |
| | PBE | 6.659 | - | - | 18.45 | 83.8 | 4.31 | 158 |
| | PBEsol | 6.600 | - | - | 17.97 | 91.2 | 4.34 | 120 |
| | SCAN | 6.613 | - | - | 18.07 | 92.0 | 4.08 | 197 |
| | Exp. [9] | 6.637 | - | - | - | - | - | - |
| | Exp. [10] | 6.628 | - | - | - | - | - | - |
| | Theo. (PBE) [3] | - | - | - | 18.45 | 83.6 | 4.2 | 159 |

**Table S3.** Frequencies of the Raman active modes (in $cm^{-1}$) for the different studied metastable Si phases obtained using various XC functionals. For each XC functional, structural geometries obtained using either SCAN or PBEsol are also used, in addition to those obtained with the same XC functional. Experimental (Exp.) values are provided as reference.

| Phase | Raman Mode | Exp. [1] | LDA | LDA (PBEsol) | LDA (SCAN) | PBE | PBE (PBEsol) | PBE (SCAN) | PBEsol | PBEsol (SCAN) |
|---|---|---|---|---|---|---|---|---|---|---|
| dc | $T_{2g}$ | 520 | 513.48 | 503.35 | 508.74 | 503.27 | 513.64 | 519.08 | 509.43 | 514.88 |
| hd | $E_{2g}$ | 496 | 492.65 | 480.64 | 486.45 | 480.13 | 492.41 | 498.27 | 488.94 | 494.81 |
| | $E_{1g}$ | 514 | 507.79 | 497.61 | 502.54 | 498.11 | 508.42 | 513.38 | 503.95 | 508.93 |
| | $A_{1g}$ | 514 | 508.03 | 498.30 | 503.43 | 498.11 | 508.53 | 513.71 | 504.20 | 509.39 |
| r8 | $A_g$ | 165 | 154.96 | 156.97 | 153.33 | 155.97 | 155.22 | 151.11 | 151.32 | 147.13 |
| | $E_g$ | 170 | 160.58 | 162.33 | 160.83 | 161.93 | 160.31 | 158.53 | 156.40 | 154.56 |
| | $A_g$ | 352 | 337.94 | 328.62 | 347.39 | 337.17 | 338.91 | 357.93 | 335.82 | 354.79 |
| | $E_g$ | 373 | 373.96 | 363.87 | 381.46 | 372.38 | 373.69 | 390.64 | 369.87 | 386.86 |
| | $A_g$ | 397 | 386.19 | 375.29 | 391.35 | 383.65 | 386.22 | 401.34 | 382.68 | 397.56 |
| | $A_g$ | 413 | 423.44 | 414.21 | 418.58 | 413.07 | 424.42 | 429.79 | 420.97 | 426.57 |
| | $E_g$ | 433 | 427.45 | 417.89 | 425.73 | 419.53 | 428.06 | 436.86 | 424.40 | 433.12 |
| | $E_g$ | 495 | 487.82 | 476.03 | 470.09 | 470.45 | 489.25 | 483.16 | 485.88 | 479.79 |
| bc8 | $T_g$ | 182 | 153.67 | 156.46 | 153.81 | 156.83 | 154.29 | 151.24 | 149.73 | 146.81 |
| | $A_g$ | 373 | 368.76 | 352.98 | 409.26 | 387.55 | 368.05 | 420.80 | 361.17 | 418.89 |
| | $T_g$ | 384 | 369.59 | 359.11 | 370.93 | 367.98 | 370.20 | 380.19 | 364.78 | 375.73 |
| | $T_g$ | 438 | 416.04 | 404.59 | 428.18 | 414.56 | 417.24 | 440.84 | 411.81 | 437.53 |
| | $E_g$ | 463 | 453.63 | 441.83 | 434.11 | 437.80 | 456.82 | 446.28 | 449.54 | 444.79 |

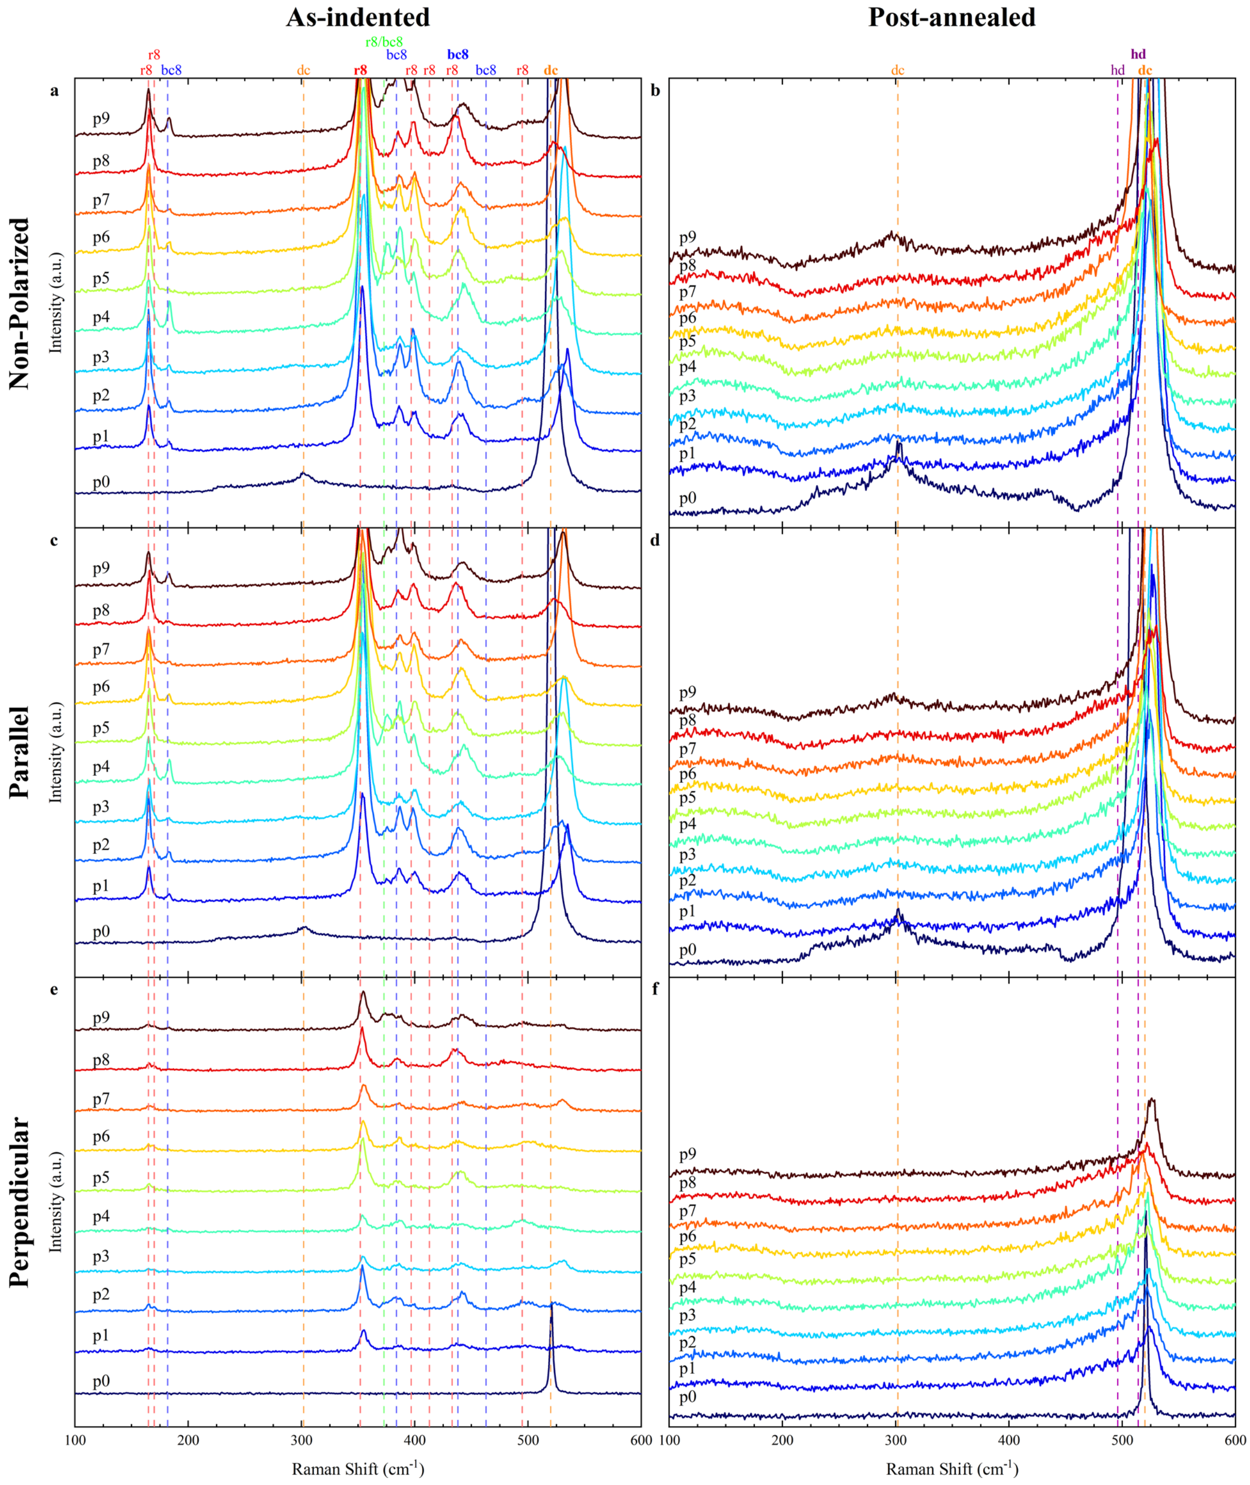


**Figure S1.** Experimental Raman spectra of (a, c, e) as-indented and (b, d, f) post-annealed silicon obtained through nanoindentation using a 20 μm tip across different scattering geometries: (a-b) Non-polarized, (c-d) Parallel, and (e-f) Perpendicular. The spectra feature distinct peaks corresponding to various silicon phases, highlighted with dashed lines: dc (orange), r8 (red), and bc8 (blue). Additionally, a Raman-active mode frequency common to both r8 and bc8 phases is marked in green. For comparison, the pristine Si (p0) spectrum is included in the graphs.

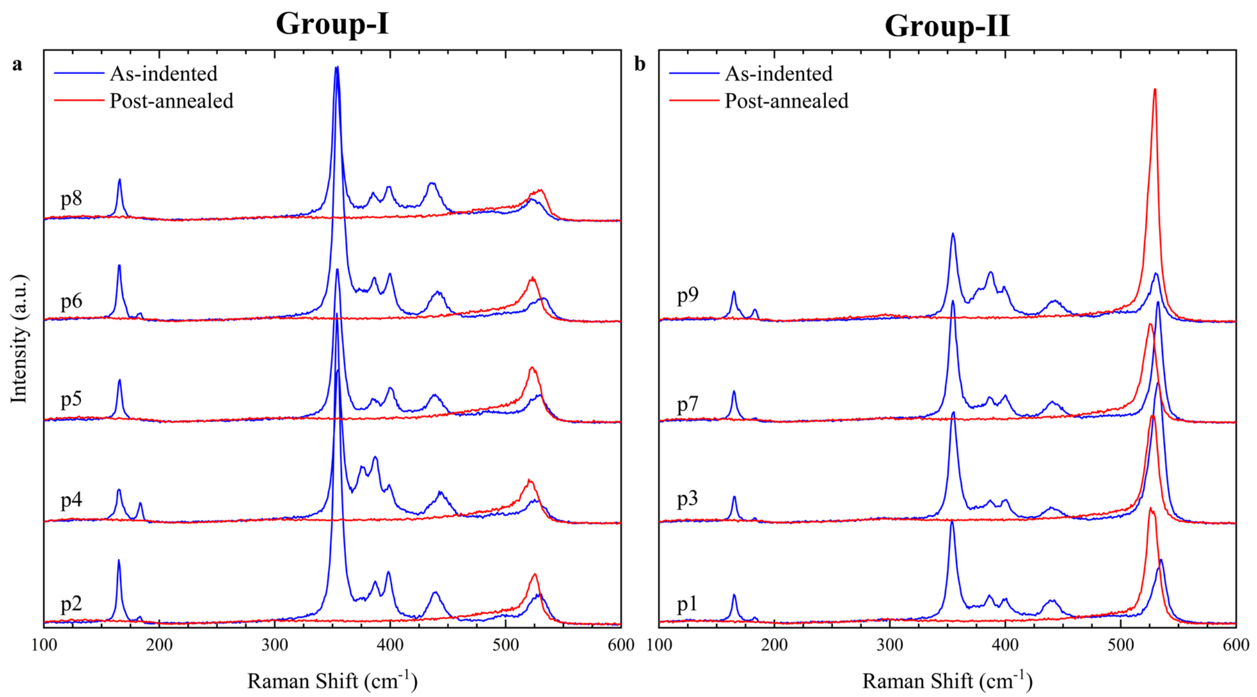


**Figure S2.** Non-polarized experimental Raman spectra of as-indented and post-annealed 20 μm tip indented silicon for: (a) Group-I and (b) Group-II.

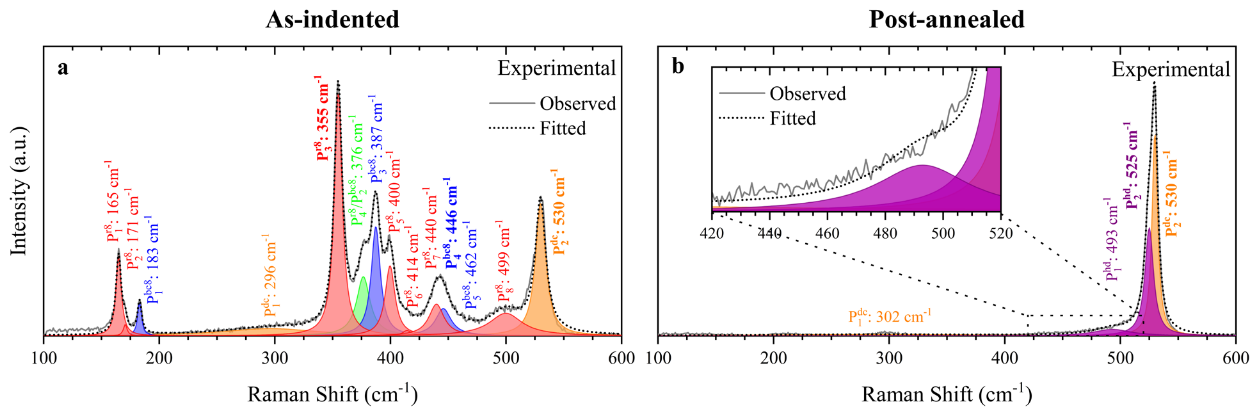


**Figure S3.** Fitted non-polarized experimental Raman spectra of 20 μm tip indented silicon pit belonging to Group-II: (a) as-indented and (b) post-annealed. Peaks associated with different metastable phases are indicated with Lorentzian functions: dc (orange), hd (purple), r8 (red), and bc8 (blue). A distinct Raman peak at 376 cm⁻¹ (green), indicative of a mixture of r8 and bc8 silicon phases, is indicated. The inset in (b) highlights the region of the experimental Raman spectra, showing the presence of the weaker $E_{2g}$ Raman peak from hd-Si.

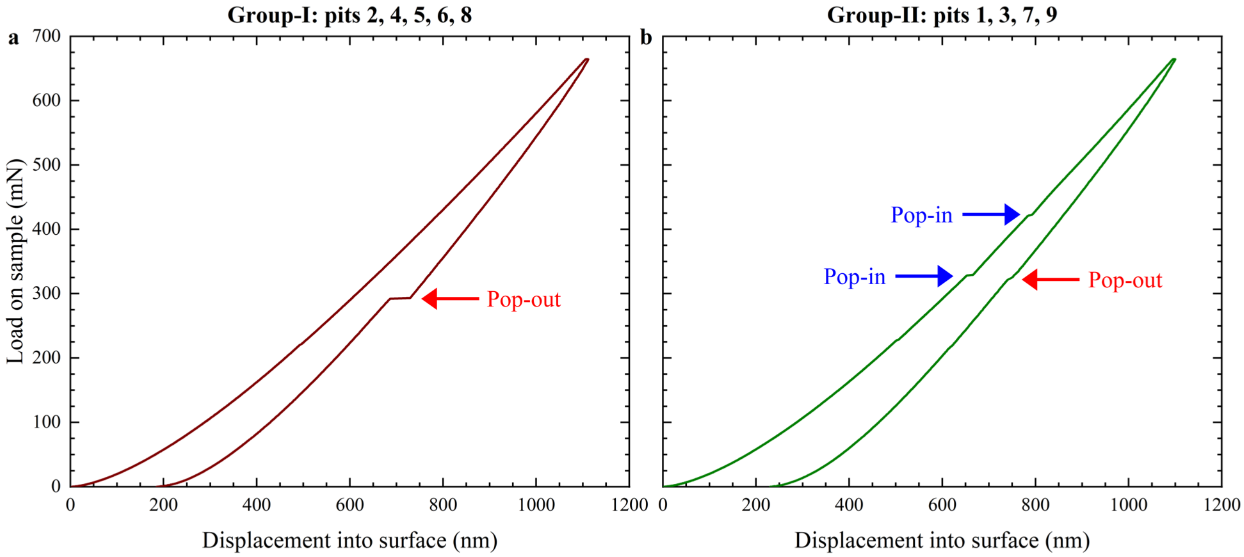


**Figure S4.** Nanoindentation load-displacement curves of silicon, loaded to a maximum of 665 mN, showing key events for: (a) Group-I and (b) Group-II. Pop-in events (blue arrow) occur during the loading segment, indicating the nucleation and propagation of crystalline defects or the formation of the metallic β-Sn phase. Pop-out events (blue arrow) in the unloading segment are typically associated with the transformation of silicon into bc8/r8 phase.

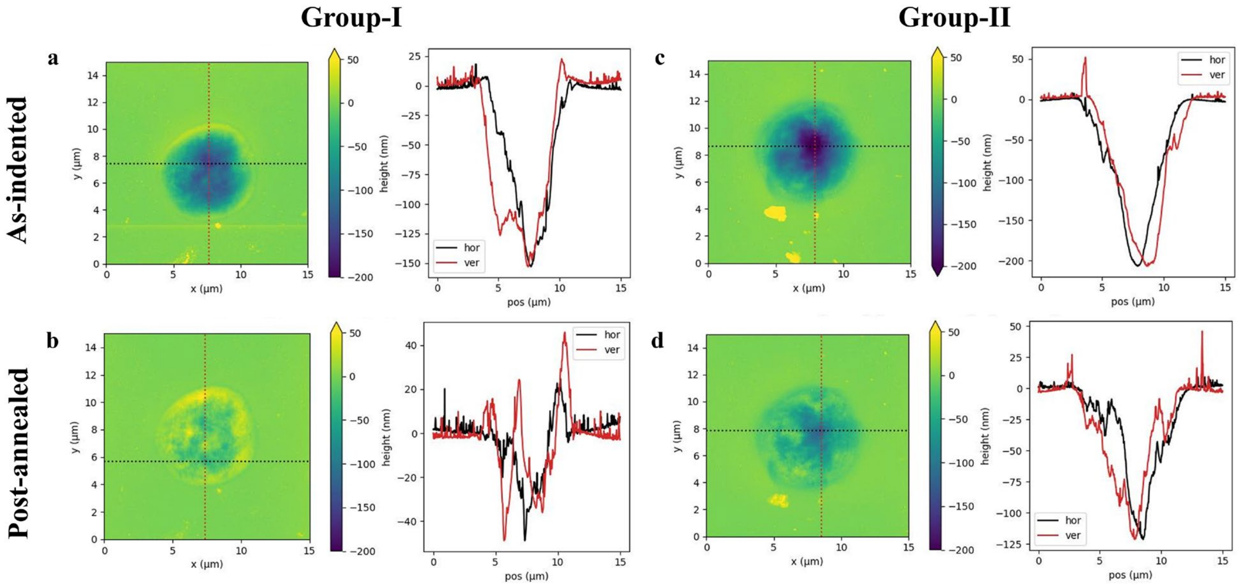


**Figure S5.** Atomic force microscopy (AFM) topography maps and corresponding cross-sectional profiles of indented silicon using a 20 μm tip. Images (a) and (c) represent the as-indented state, while (b) and (d) show the post-annealed state for two distinct groups of pits: Group-I (a-b) and Group-II (c-d). In the as-indented condition, Group-I pits show a shallower indentation (150 nm) compared to Group-II pits (200 nm). After annealing, Group-I pits exhibit maximal depth change (110 nm) in contrast to Group-II pits (75 nm).

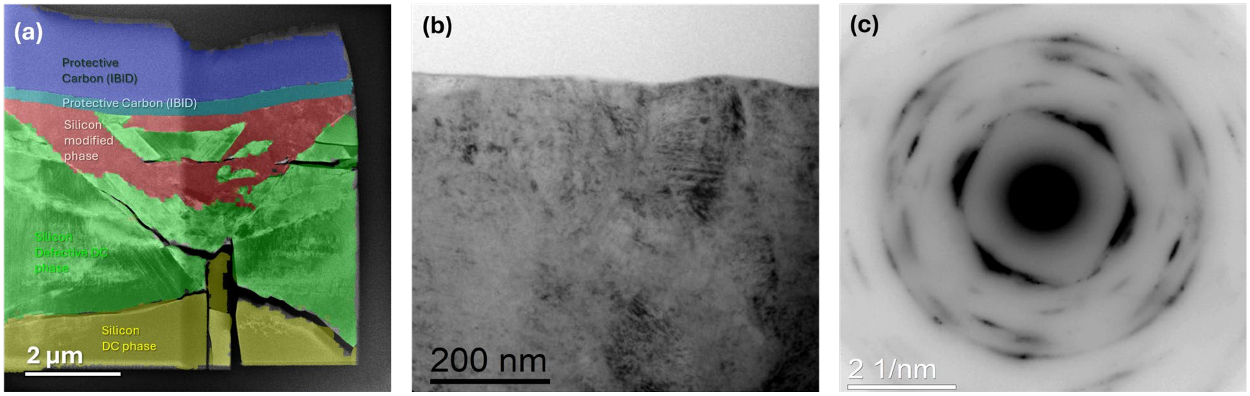


**Figure S6.** Cross-sectional analysis of the indented silicon using 10 µm tip. (a) Focused ion beam (FIB) cross-section of the indented area showing different silicon phases and protective carbon layers. The silicon is divided into a crystalline dc phase, a defective dc phase, and a modified silicon phase near the indentation site, with a protective carbon layer deposited via ion beam-induced deposition (IBID) on the surface. (b) High-resolution transmission electron microscopy (HRTEM) image of the indented silicon region, revealing disordered structures and defects induced by nanoindentation. (c) Selected area electron diffraction (SAED) pattern of the modified silicon phase, displaying characteristic ring patterns indicative of its crystalline and defect structure.

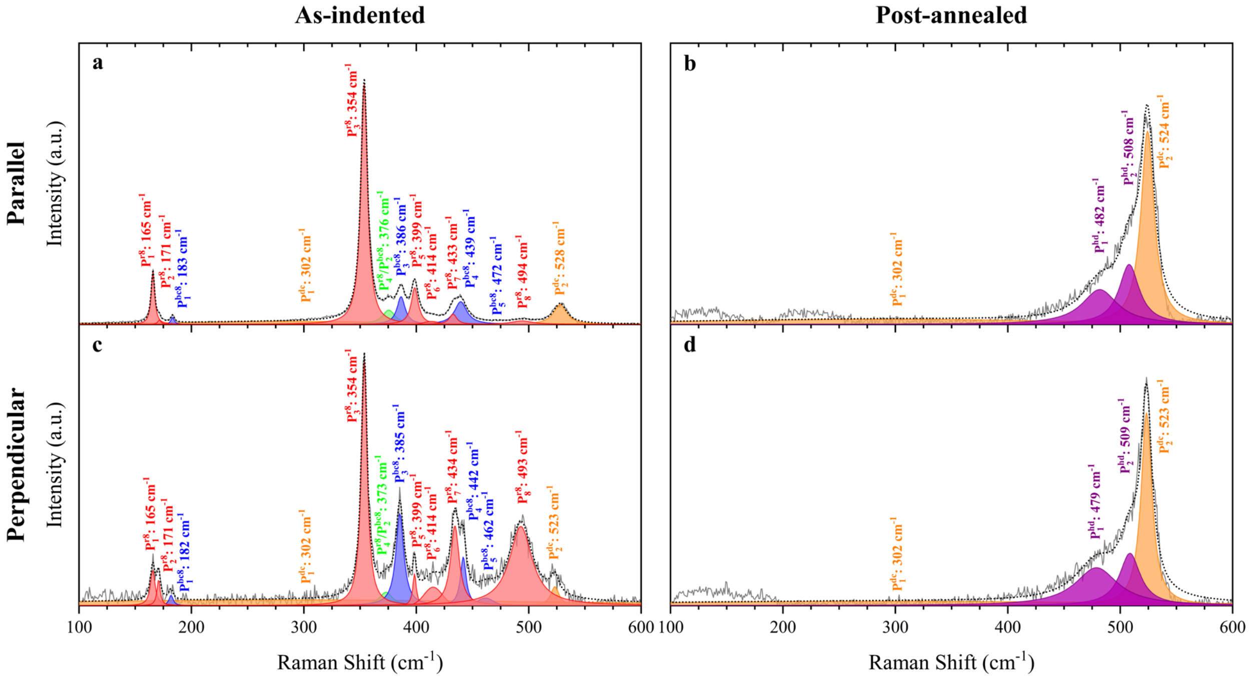


**Figure S7.** Fitted polarized experimental Raman spectra of (a, c) as-indented and (b, d) post-annealed 10 µm tip indented silicon across different scattering geometries: (a-b) Parallel and (c-d) Perpendicular. Peaks associated with different metastable phases are indicated with Lorentzian functions: dc (orange), hd (purple), r8 (red), and bc8 (blue). Additionally, a Raman-active mode frequency common to both r8 and bc8 phases is marked in green.

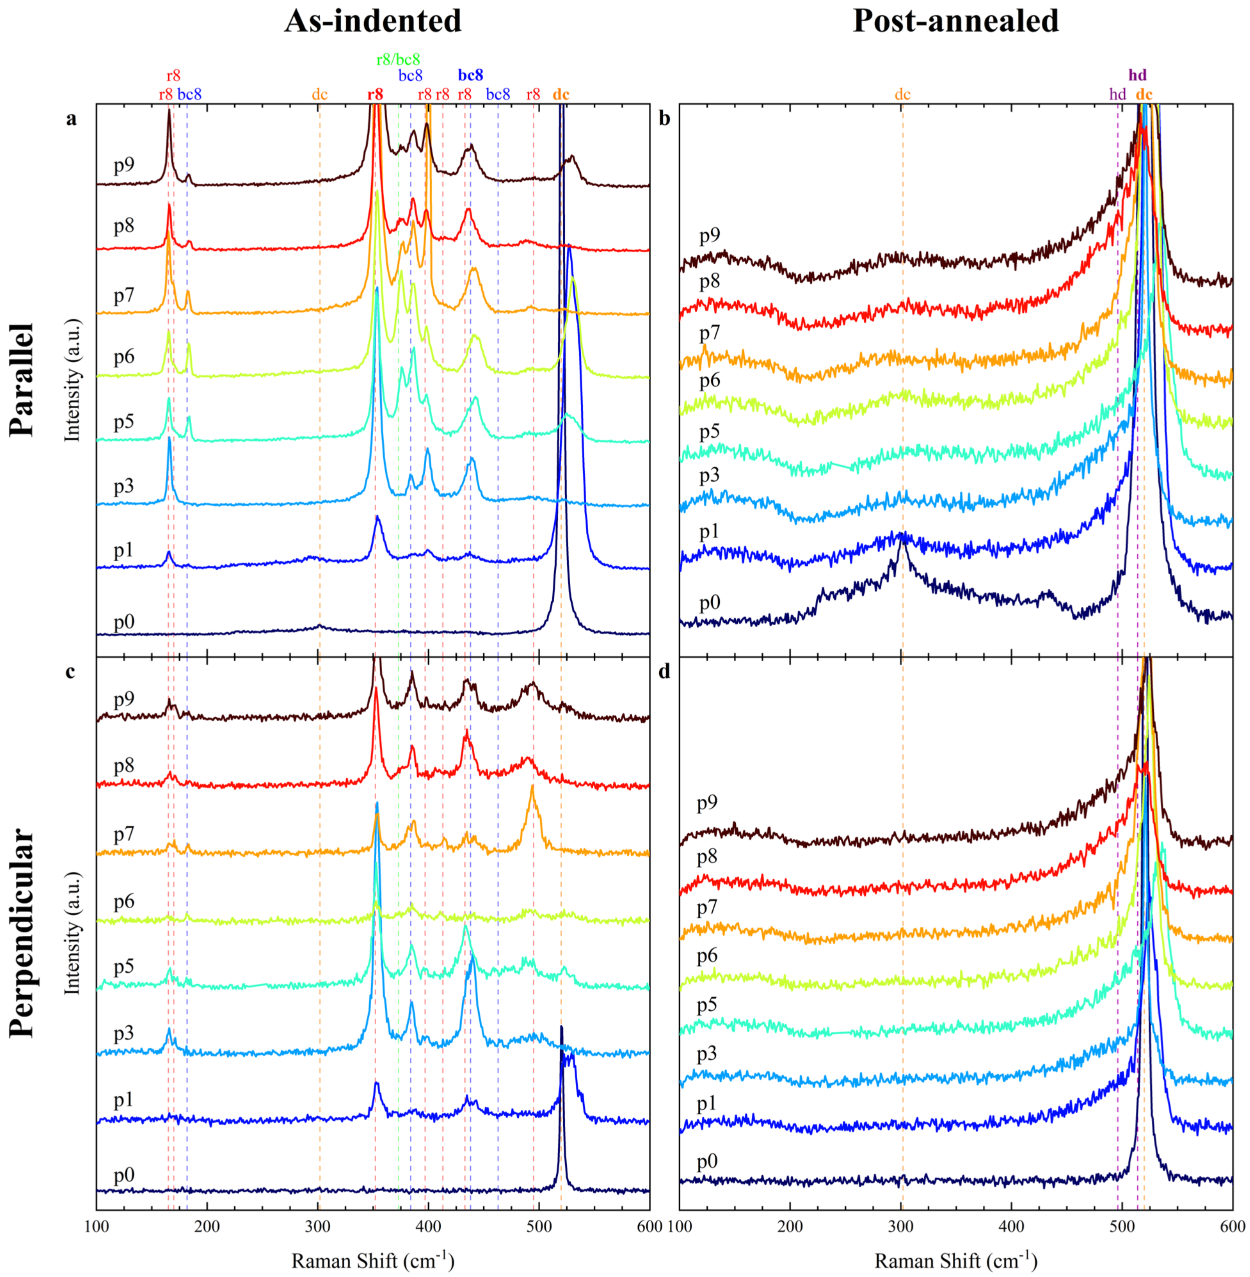


**Figure S8.** Experimental Raman spectra of (a, c) as-indented and (b, d) post-annealed 10 µm tip indented silicon across different scattering geometries: (a-b) Parallel and (c-d) Perpendicular. The spectra feature distinct peaks corresponding to various silicon phases, highlighted with dashed lines: dc (orange), r8 (red), and bc8 (blue). Additionally, a Raman-active mode frequency common to both r8 and bc8 phases is marked in green. For comparison, the pristine Si (p0) spectrum is included in the graphs.

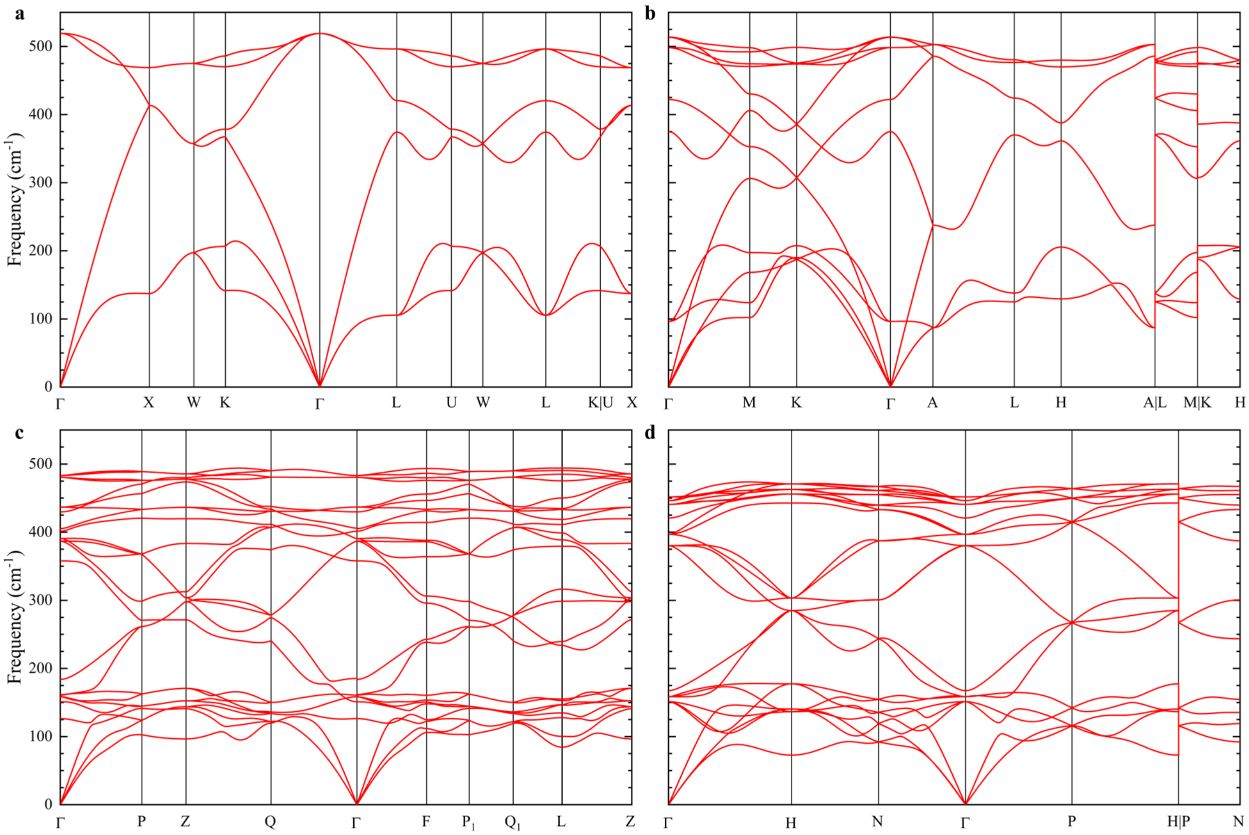


**Figure S9.** Calculated phonon dispersions by Density Functional Perturbation Theory (DFPT) of different silicon phases: (a) dc, (b) hd, (c) r8, and (d) bc8.

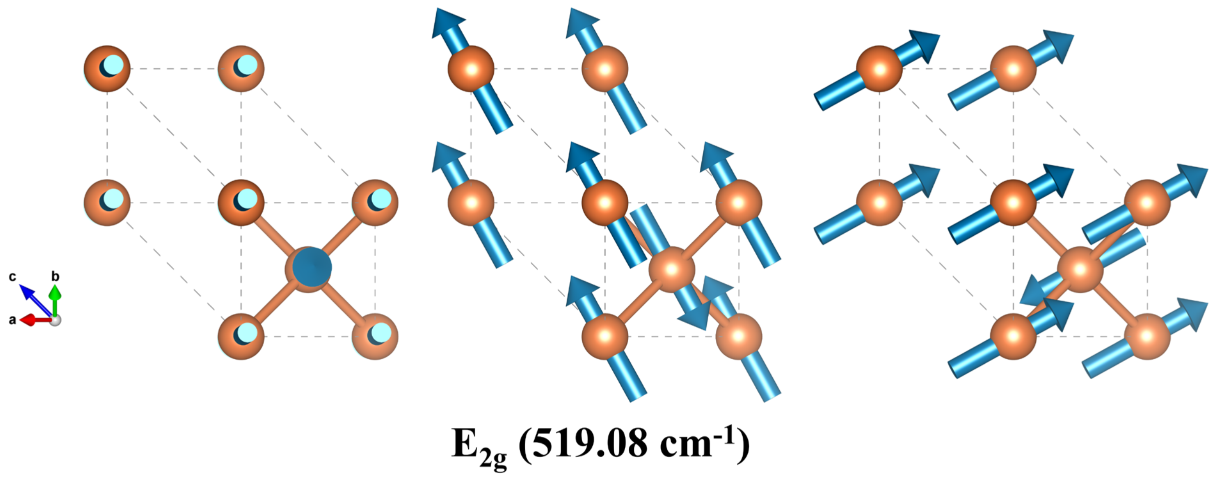


**Figure S10.** Visual representations of the Raman-active phonon modes in the dc phase of silicon. Blue arrows indicate the direction of atomic displacements. The dashed grey lines outline the primitive unit cell. The lengths of the arrows are proportional to the square roots of the vibration amplitudes.

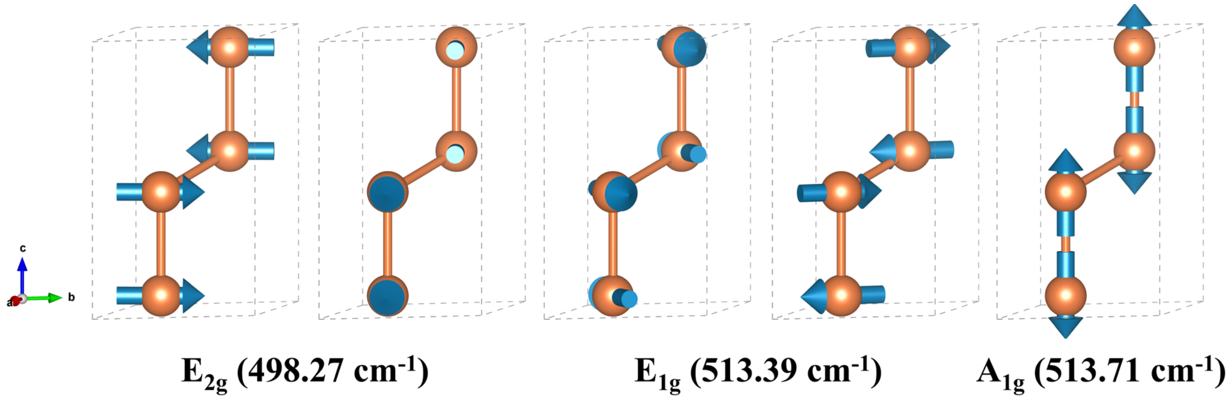


**Figure S11.** Visual representations of the Raman-active phonon modes in the hd phase of silicon. Blue arrows indicate the direction of atomic displacements. The dashed grey lines outline the primitive unit cell. The lengths of the arrows are proportional to the square roots of the vibration amplitudes.

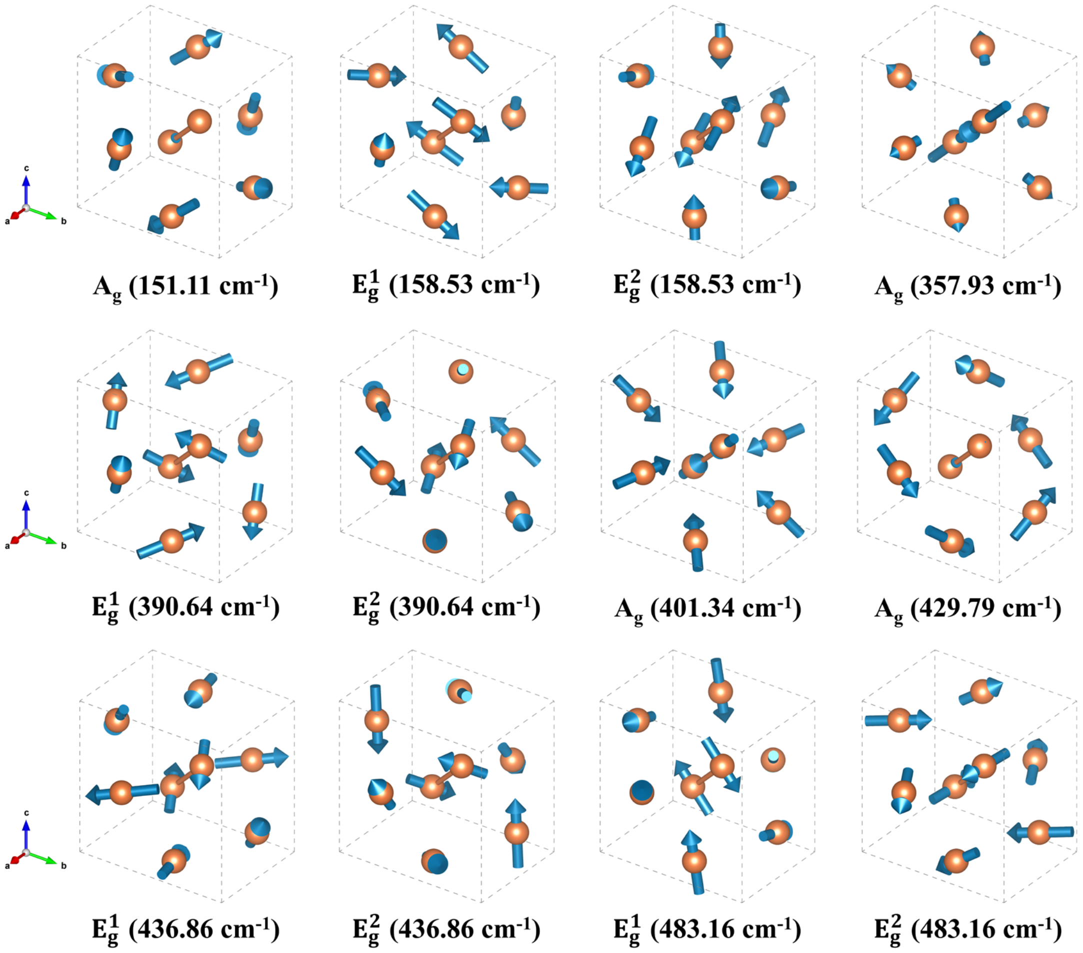


**Figure S12.** Visual representations of the Raman-active phonon modes in the r8 phase of silicon. Blue arrows indicate the direction of atomic displacements. The dashed grey lines outline the primitive unit cell. The lengths of the arrows are proportional to the square roots of the vibration amplitudes.

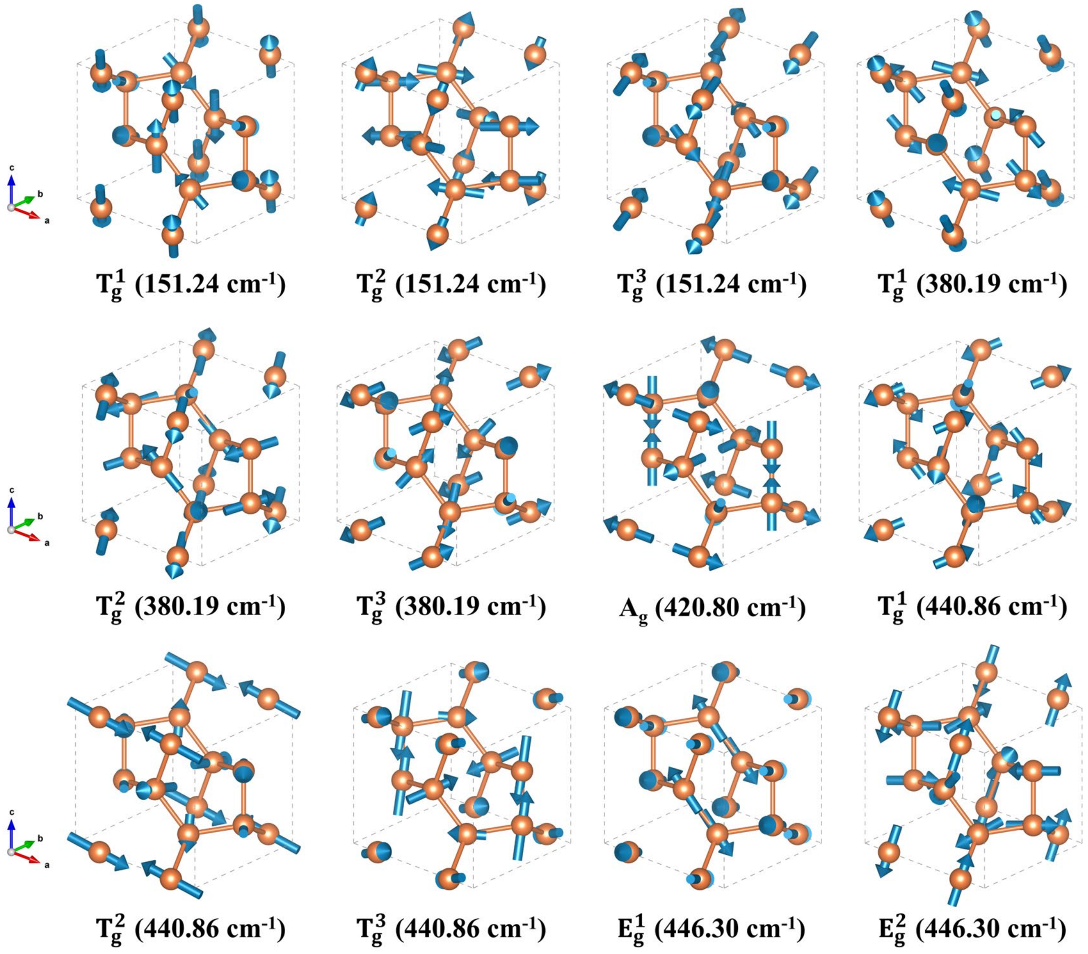


**Figure S13.** Visual representations of the Raman-active phonon modes in the bc8 phase of silicon. Blue arrows indicate the direction of atomic displacements. The dashed grey lines outline the primitive unit cell. The lengths of the arrows are proportional to the square roots of the vibration amplitudes.

## References:


[1] S. Wong, B. C. Johnson, B. Haberl, A. Mujica, J. C. McCallum, J. S. Williams, and J. E. Bradby, Thermal evolution of the indentation-induced phases of silicon, Journal of Applied Physics **126**, 105901 (2019).

[2] *Numerical data and functional relationships in science and technology. Teilbd. a: Gruppe 3: Kristall- und Festkörperphysik = Group 3: @Crystal and solid state physics Bd. 16. Neubearbeitung u. Erweiterung d. Bd. 3,3 u. 3,9, Ferroelektrika und verwandte Substanzen / T. Mitsui; S. Nomura Oxide*, Vol. 16 (Springer, Berlin Heidelberg, 1981).

[3] A. Mujica, C. J. Pickard, and R. J. Needs, Low-energy tetrahedral polymorphs of carbon, silicon, and germanium, Phys. Rev. B **91**, 214104 (2015).

[4] C. Raffy, J. Furthmüller, and F. Bechstedt, Properties of hexagonal polytypes of group-IV elements from first-principles calculations, Phys. Rev. B **66**, 075201 (2002).

[5] H. I. T. Hauge et al., Hexagonal Silicon Realized, Nano Lett. **15**, 5855 (2015).

[6] H. S. Ahn, S.-W. Kim, G. S. Lee, K. H. Kim, J. H. Lee, D. H. Ha, Y. T. Chun, and S. Ryu, Optical property of hexagonal (2H) silicon crystal, Semicond. Sci. Technol. **36**, 095023 (2021).

[7] Y. Zhang, Z. Iqbal, S. Vijayalakshmi, and H. Grebel, Stable hexagonal-wurtzite silicon phase by laser ablation, Applied Physics Letters **75**, 2758 (1999).

[8] J. M. Besson, E. H. Mokhtari, J. Gonzalez, and G. Weill, Electrical properties of semimetallic silicon III and semiconductive silicon IV at ambient pressure, Phys. Rev. Lett. **59**, 473 (1987).

[9] R. O. Piltz, J. R. Maclean, S. J. Clark, G. J. Ackland, P. D. Hatton, and J. Crain, Structure and properties of silicon XII: A complex tetrahedrally bonded phase, Phys. Rev. B **52**, 4072 (1995).

[10] H. Zhang, H. Liu, K. Wei, O. O. Kurakevych, Y. Le Godec, Z. Liu, J. Martin, M. Guerrette, G. S. Nolas, and T. A. Strobel, BC8 Silicon (Si-III) is a Narrow-Gap Semiconductor, Phys. Rev. Lett. **118**, 146601 (2017).
